# Supplementary material for: Quasi-static responses of marine mussel plaques attached to deformable wet substrates under directional tensions
Source: arXiv:2305.15129 source file (2023-10-24)
Supplement: Supplementary file 1 [file Supplementary_Information.pdf]

# Supplementary Information

## Quasi-static responses of marine mussel plaques detached from deformable wet substrates under directional tensions

Yong Pang<sup>1</sup>, Tao Liu<sup>1, \*</sup>

<sup>1</sup>School of Engineering and Materials Science, Queen Mary University of London, London E1 4NS, UK

\*Corresponding author: Tao Liu, e-mail: [tao.liu@qmul.ac.uk](mailto:tao.liu@qmul.ac.uk)

### **This PDF file includes the following:**

Supplementary Text

Supplementary Figures 1 to 12

Supplementary Tables 1 to 2

## S1. Details on mussel samples preparation

In this section, details on mussel sample preparation have been presented. Figure S1a shows that the blue mussels were collected from the intertidal zone of the Hunstanton mussel farm (52.94 °N, 0.49 °E). These mussel samples were placed in the laboratory aquarium system (Figure S1b), which includes a fish tank, a wave maker, an air pump, a water pump, and an aquarium chiller. Once the marine mussels were fully acclimated to the laboratory environment, sixteen adult mussels of a similar size were fastened with substrate checkerboard using rubber bands. Each checkerboard was filled with four-by-four substrates (Figure S1c) with the same stiffness to allow plaque deposition. The deposited plaque-tread systems were carefully cut for mechanical tests and SEM imaging.

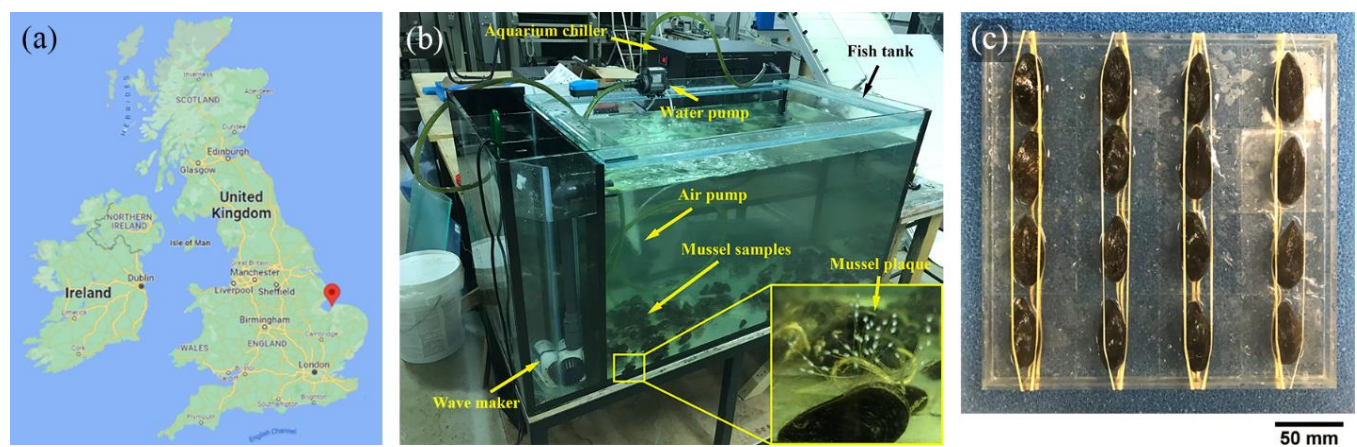

**Figure S1. Preparation of marine mussel samples.** (a) Marine mussels were collected from Hunstanton mussel farm (52.94 °N, 0.49 °E). (b) Laboratory aquarium system to simulate the natural environment of mussel habitat. (c) Four by four substrate checkerboard was used for the mechanical tests. Marine mussels with consistent size were fastened with substrates using rubber bands.

## S2. Details on PDMS substrates fabrication

Sylgard 184 silicone elastomer (10:1 wt% for base and curing agent) and Sylgard 527 silicone gel (1:1 wt% for parts A and B) were mixed with different mass ratios to tune Young's modulus of the substrate. Table S1 shows the details of the synthesis of different PDMS formulations. Four mass ratios of Sylgard 184 to 527 (ranging from 1:0, 4:1, 3:2, and 2:3) were employed to design the substrates. These raw compounds of PDMS were mixed for 15 minutes using a magnetic stirrer and degassed in a vacuum oven for 30 minutes to remove air bubbles. Then, the degassed PDMS was filled into moulds of standard tensile specimens in accordance with ASTM D412 [1] (Figure S2a). Subsequently, these moulds were cured in

an oven at 65°C, which is sufficient to cure these PDMS for 24 hours. Finally, the PDMS uniaxial tensile specimens were tested on an Instron 5966 universal testing system at a 1% strain rate (quasi-static tests) to measure their stiffness. Five tensile specimens were tested in each PDMS blend to ensure high repeatability and accuracy of uniaxial tensile tests.

**Table S1.** PDMS formulations for the development of PDMS substrates with tunable stiffness

| Substrates<br>stiffness | Sylgard 184 (g) |              |          | Sylgard 527 (g) |        |          | Sylgard 184: Sylgard 527<br>(Mass ratio) |
|-------------------------|-----------------|--------------|----------|-----------------|--------|----------|------------------------------------------|
|                         | Base            | Curing agent | Subtotal | Part A          | Part B | Subtotal |                                          |
| 1.68 MPa                | 18.18           | 1.82         | 20.00    | 0.00            | 0.00   | 0.00     | 1:0                                      |
| 1.34 MPa                | 14.55           | 1.45         | 16.00    | 2.00            | 2.00   | 4.00     | 4:1                                      |
| 0.96 MPa                | 10.91           | 1.09         | 12.00    | 4.00            | 4.00   | 8.00     | 3:2                                      |
| 0.57 MPa                | 7.27            | 0.73         | 8.00     | 6.00            | 6.00   | 12.00    | 2:3                                      |

**Table S2.** Spin speed and coating duration were used for different PDMS substrates.

| Stiffness  | Substrate layers | Thickness ( $\mu\text{m}$ ) | Spin speed (rpm) | Duration (s) |
|------------|------------------|-----------------------------|------------------|--------------|
| E=1.68 MPa | PDMS layer       | 100×2                       | 800              | 30           |
|            | Particle layer   | 15                          | 2100             | 260          |
|            | Pigment layer    | 15                          | 2100             | 260          |
| E=1.34 MPa | PDMS layer       | 100×2                       | 550              | 30           |
|            | Particle layer   | 15                          | 2000             | 240          |
|            | Pigment layer    | 15                          | 2000             | 240          |
| E=0.96 MPa | PDMS layer       | 100×2                       | 500              | 30           |
|            | Particle layer   | 15                          | 1600             | 220          |
|            | Pigment layer    | 15                          | 1600             | 220          |
| E=0.57 MPa | PDMS layer       | 100×2                       | 450              | 30           |
|            | Particle layer   | 15                          | 1400             | 200          |
|            | Pigment layer    | 15                          | 1400             | 200          |

Figures S2 b to e show the engineering stress-strain curves of different PDMS blends. The mechanical behaviours of different PDMS formulations mainly exhibit a linear stage followed by a non-linear stage. The results of uniaxial tensile tests suggest that Young's moduli of different PDMS formulations range from 0.57 to 1.68 MPa. These elastic properties were further employed to investigate the effects of substrate stiffness on plaque detachment. PDMS substrates were spin-coated layer upon layer to achieve a multi-layer structure (Figure 2a). To achieve a consistent PDMS thickness, different spin speeds corresponding to PDMS formulations were employed (Table S2). Here, the PDMS layer was coated twice to form a 200  $\mu\text{m}$  thickness which ensures mechanical properties of the PDMS layer are thickness independent [2].

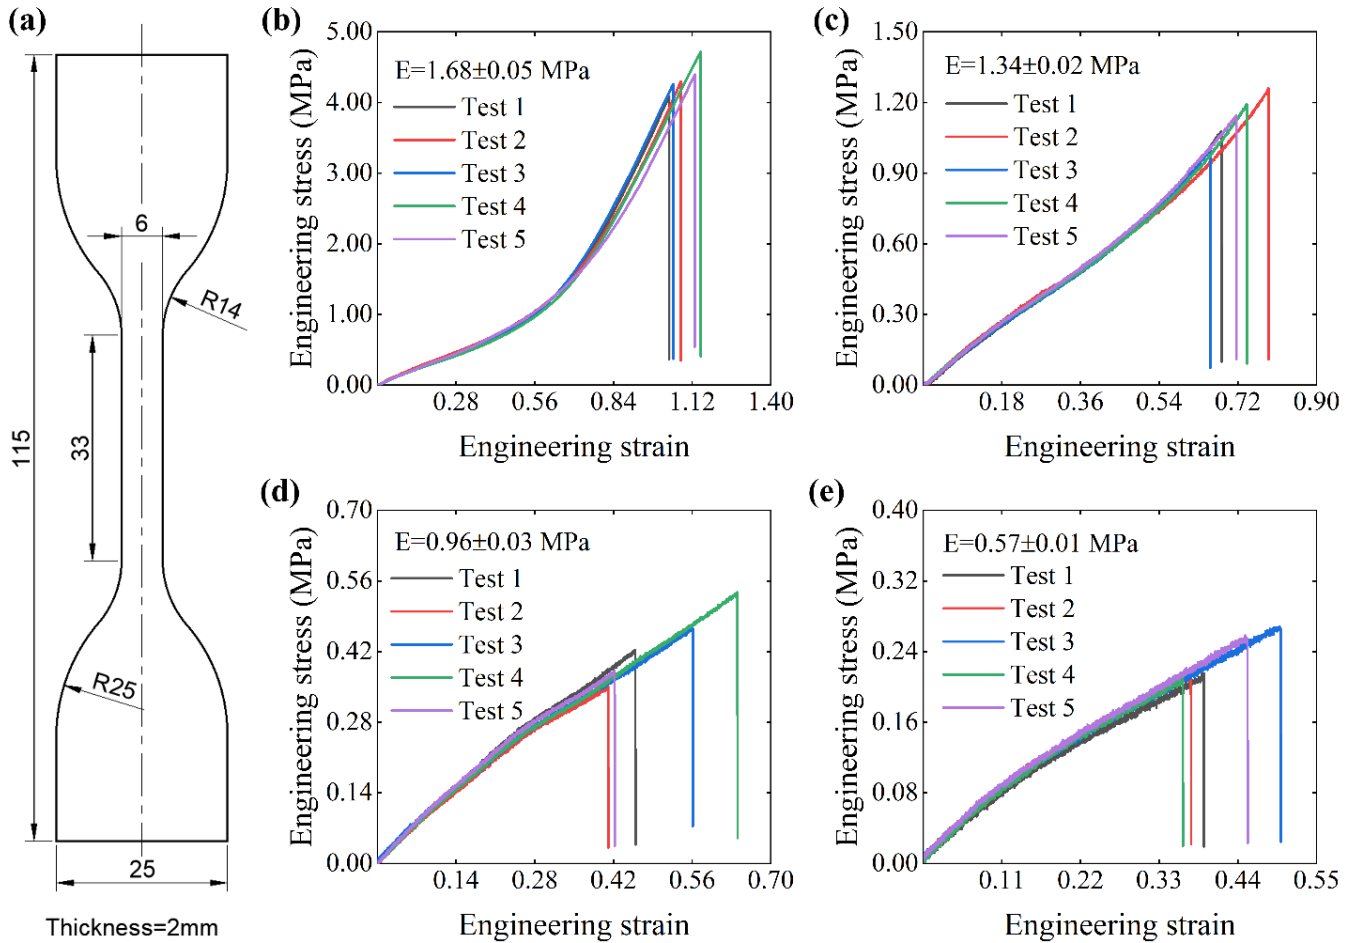

**Figure S2. Mechanical properties of different PDMS formulations.** (a) Dimensions of standard uniaxial tensile specimen in accordance with ASTM D412-16. (b-e) Stress-strain curves (n=5) of different PDMS formulations.

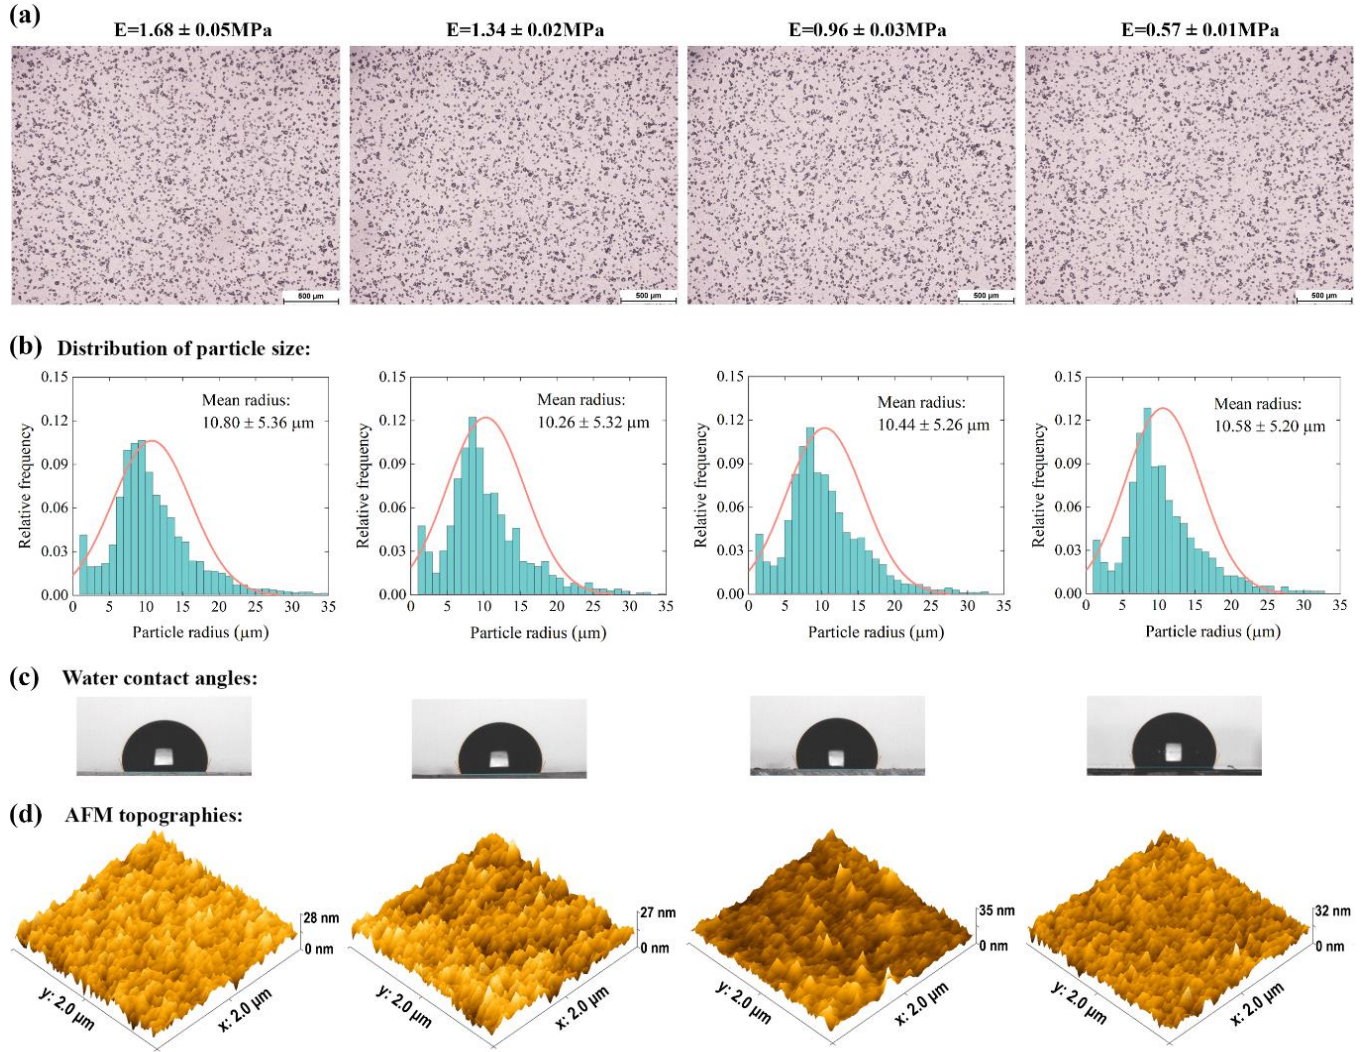

**Figure S3. Surface conditions of substrates with different stiffness.** (a) Representative patterns of microparticles in different PDMS substrates, (b) distribution of microparticle sizes, (c) water contact angles, and (d) AFM topography.

Since the surface conditions of substrates could affect the plaque detachment [3-5], micro-particle size, wettability and surface roughness of different PDMS substrates were investigated. Figure S3 shows the surface conditions of substrates with different stiffness. The proposed optical microscopy was employed to image these randomly distributed microparticles (Figure S3a), and ImageJ was employed to analyze the particle size and distribution [6]. The particle size follows a normal distribution in all substrates, and the mean values of the particle radius are between  $10.26 \pm 5.32 \mu\text{m}$  and  $10.80 \pm 5.36 \mu\text{m}$  (Figure S3b), which indicates that there are no significant differences between different substrates in terms of particle size and distribution. To further confirm the wettability and the surface roughness of PDMS substrates, water

contact angles (WCAs) and 3D surface topographies of different substrates were characterized. The WCAs of these four substrates are highly consistent and fall in the range of  $108.50^\circ \pm 2.84^\circ$  and  $112.0^\circ \pm 3.42^\circ$ , which suggests that the proposed PDMS substrates behave with a similar wettability. The surface roughness of the proposed substrates was measured by atomic force microscopy (AFM). The root-mean-square roughness (Rq) was  $3.08 \pm 0.28$  nm,  $3.74 \pm 0.23$  nm,  $3.73 \pm 0.25$  nm, and  $3.46 \pm 0.27$  nm, respectively. The variation in surface roughness was less than 1nm, which indicates that these PDMS substrates have a similar surface roughness. In each set of PDMS substrates, WCA and surface roughness were measured by taking the average of five individual readings. Figures S3 c and d show the representative WCAs and surface roughness of different PDMS substrates, respectively. Therefore, the proposed substrates were employed to ensure a consistency in surface roughness and wettability, which allows the relationship between substrate stiffness and plaque adhesive property to be well understood.

#### S4. Details on mechanical tests

The mechanical tests of plaque detachment were conducted on a customized optical microscopy system (Figure S4). The substrate was placed at the centre of a transparent acrylic plate and fixed by a rigid microscope slide holder (the inset of Figure S4b). To apply the directional tensile load, the mussel thread was clamped by a soft tip tweezer (the inset of Figure S4b), which ensures that there is no damage to the thread and no sliding between the thread and the tweezer. The tweezer was attached to a high-resolution load cell (Honeywell Model 34) with a precision of 10 mN for force measurement. The voltage signal from the load cell was first amplified by an AD620 amplifier and then calibrated using standard weights. The tweezer and load cell were placed in series with a linear actuator (Thomson MLA11A05) which is controlled by a custom-written Adriano program via a motor controller (Kollmorgen P5000) (Figure S4b). Two power suppliers were employed for the system, 5V to power the load cell and 30V to power the linear actuator (Figure S4a). A customized imaging system, including a  $12\times$  macro zoom lens (NAVITAR 1-50486D), a CCD camera (Pixelink PL-D753MU,  $1936 \times 1464$  pixels), a LED illuminator (Edmund Optics, 530 nm), a non-polarizing splitter (Thorlabs CCM1-BS013/M, 50:50 split ratio) and a positioning stage was placed below the substrate to capture the plaque/substrate deformation (the inset of Figure S4a). In addition, another  $12\times$  zoom lens and CCD camera were employed to provide the side view of plaque deformation under tensile loads (Figure S4b). Figures S5 a-d show the representative surface traction ( $T$ ) - total strain ( $\epsilon_t$ ) curves of plaque detachment at various combinations of pulling angle and substrate stiffness. Five individual maximum tractions were averaged at each pulling angle and plotted in Figure 4c.

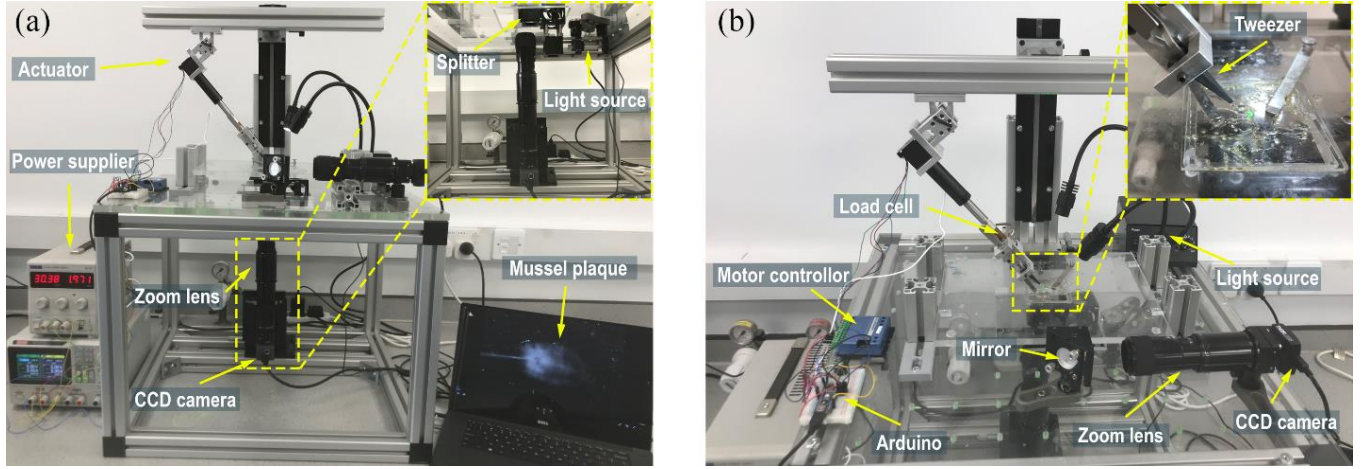

**Figure S4.** Experimental set-up for the mechanical tests. (a) Side view of the customized optical system. (b) Top view of the customized optical system.

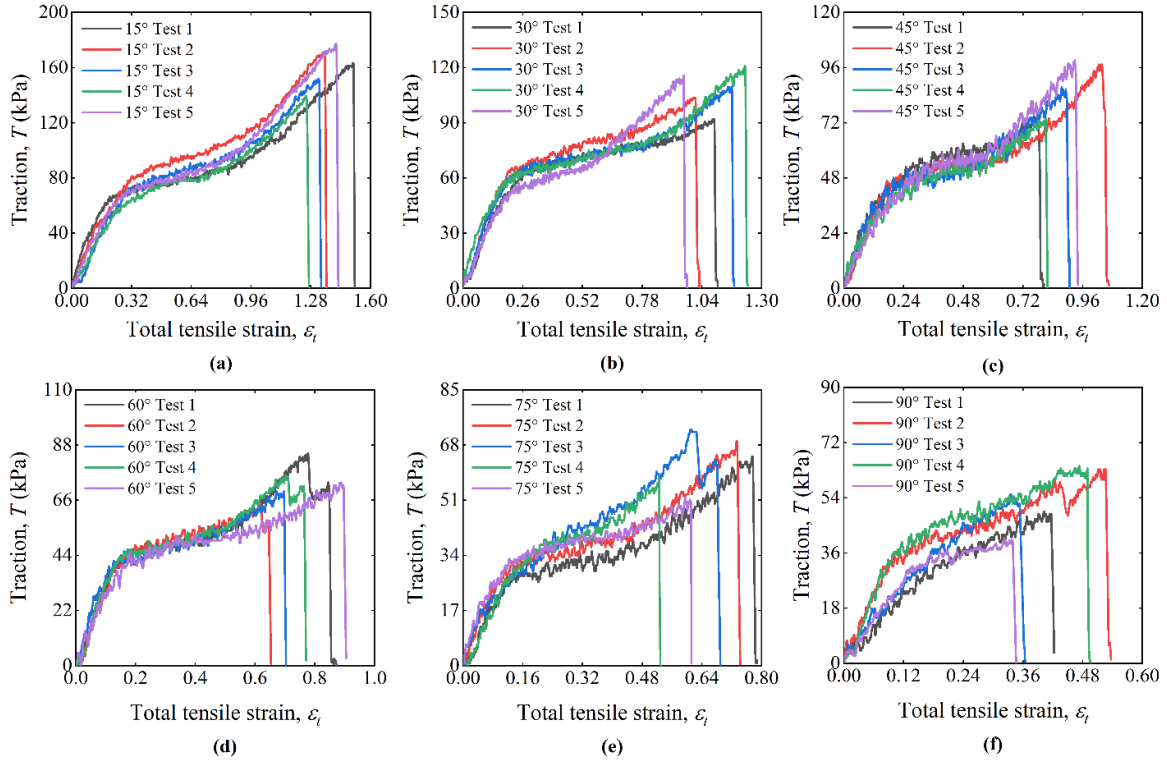

**Figure S5.** Surface traction ( $T$ ) - total strain ( $\epsilon_t$ ) curves of plaque detachment from the substrate (Stiffness  $E = 3$  GPa). (a) - (f) directional tensions at pulling angles ranging from  $15^\circ$  to  $90^\circ$  at an increment of  $15^\circ$ , respectively.

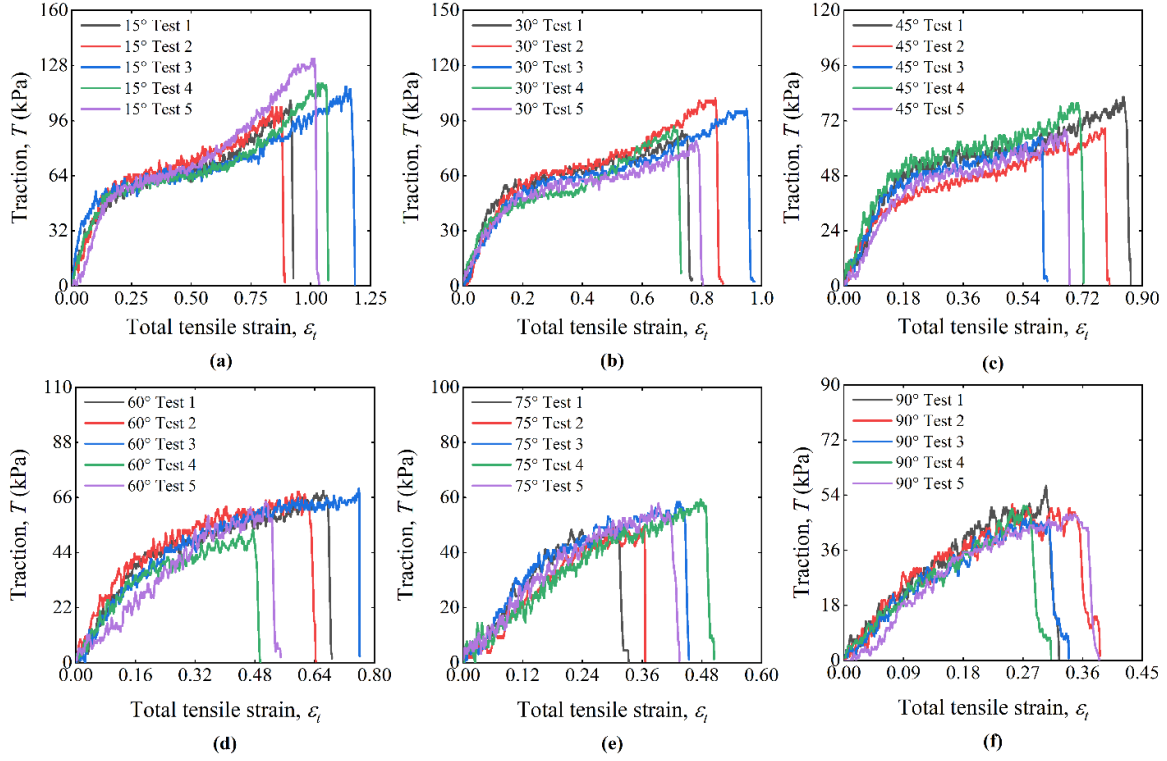

**Figure S6.** Surface traction ( $T$ ) - total strain ( $\epsilon_t$ ) curves of plaque detachment from the substrate (Stiffness  $E = 1.68$  MPa). (a) - (f) directional tensions at pulling angles ranging from 15° to 90° at an increment of 15°, respectively.

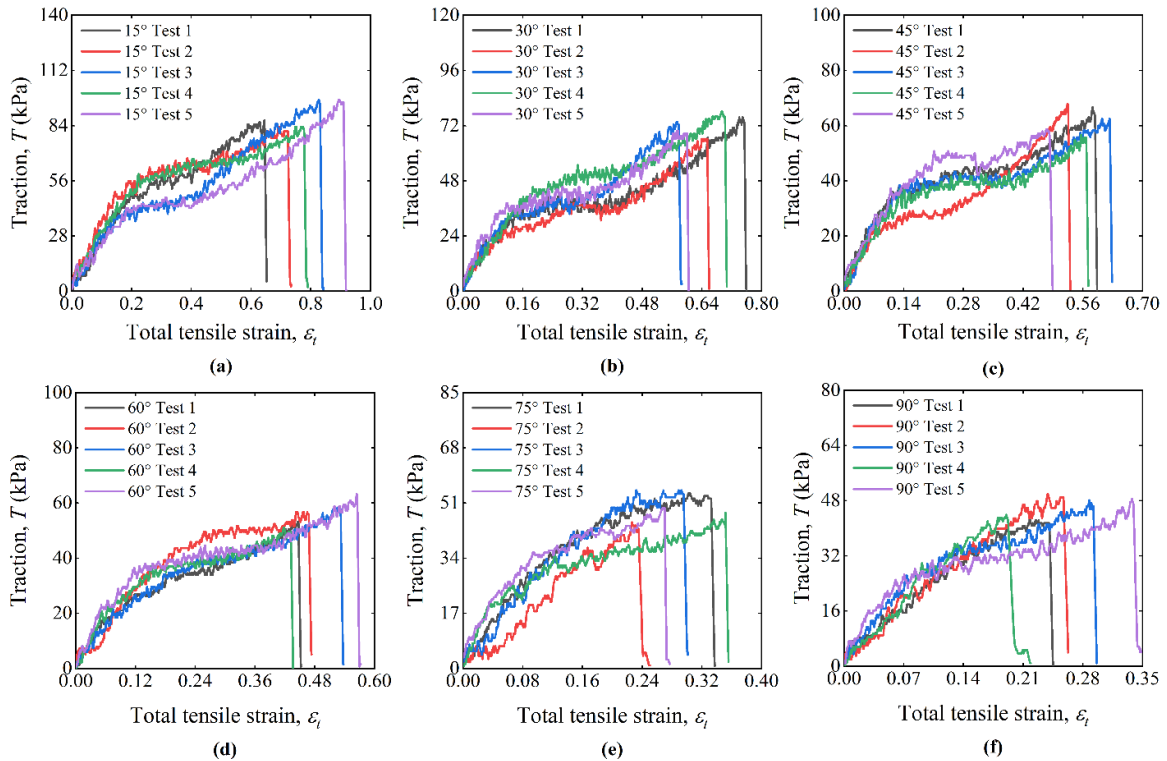

**Figure S7.** Surface traction ( $T$ ) - total strain ( $\epsilon_t$ ) curves of plaque detachment from the substrate (Stiffness  $E = 1.34$  MPa). (a) - (f) directional tensions at pulling angles ranging from 15° to 90° at an increment of 15°, respectively.

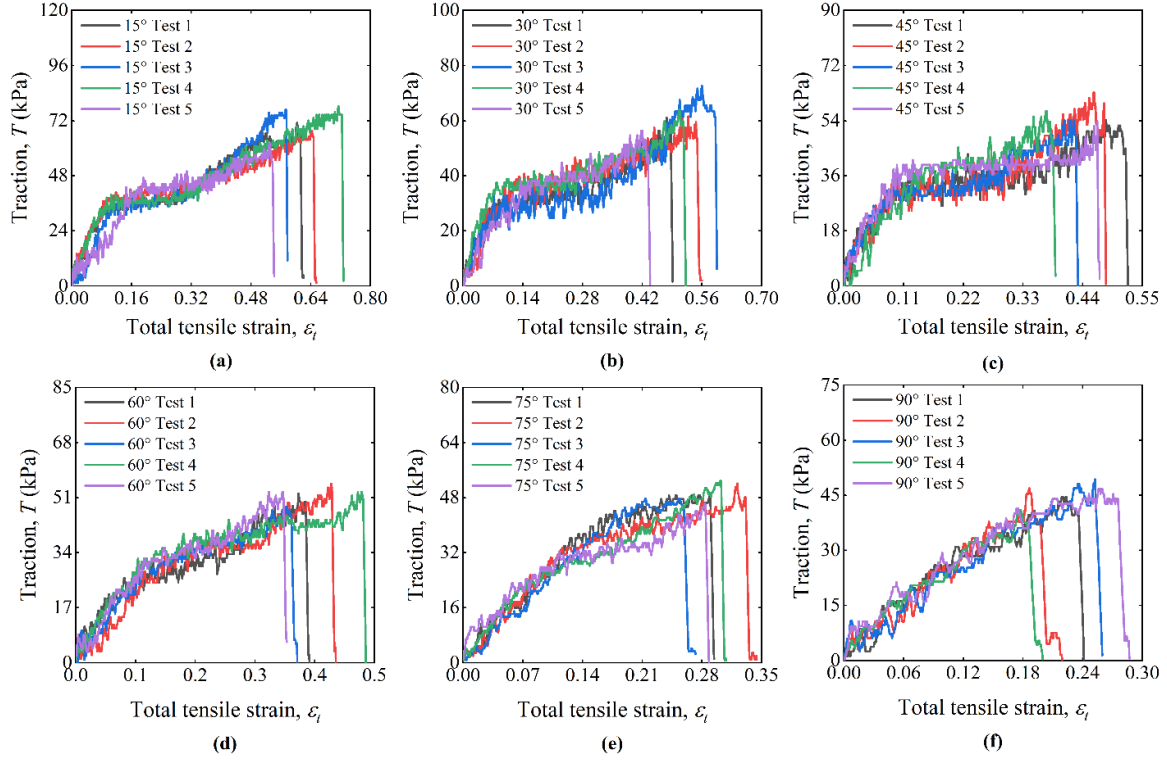

**Figure S8.** Surface traction ( $T$ ) - total strain ( $\epsilon_t$ ) curves of plaque detachment from the substrate (Stiffness  $E = 0.96$  MPa). (a) - (f) directional tensions at pulling angles ranging from  $15^\circ$  to  $90^\circ$  at an increment of  $15^\circ$ , respectively.

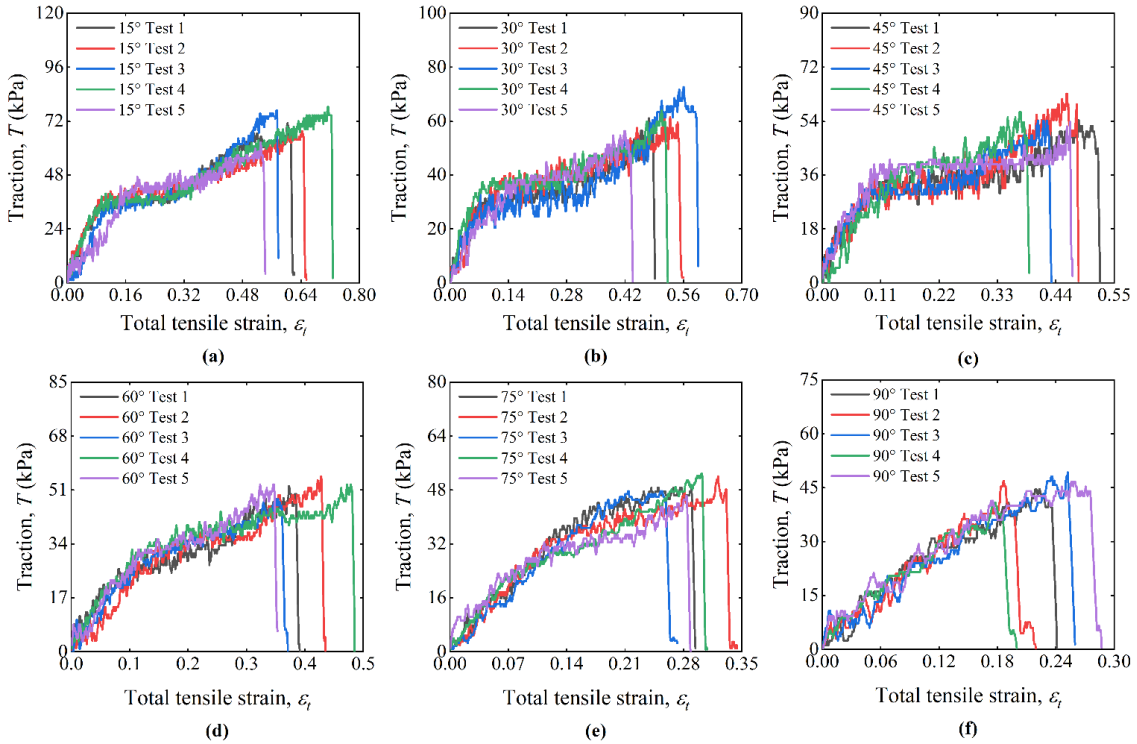

**Figure S9.** Surface traction ( $T$ ) - total strain ( $\epsilon_t$ ) curves of plaque detachment from the substrate (Stiffness  $E = 0.57$  MPa). (a) - (f) directional tensions at pulling angles ranging from  $15^\circ$  to  $90^\circ$  at an increment of  $15^\circ$ , respectively.

## S5. Details on plaque and substrate interactions

Figures S10 and S11 show the side view of plaque deformation, the in-plane principal strains ( $\varepsilon_{max}$  and  $\varepsilon_{min}$ ) and FE-predicted interface damage for the plaques detached under 45° tension from “stiff” and “soft” substrate, respectively. Here, substrates deformation at “stiff” and “soft” substrates are fairly similar. Both FE simulation and in-situ DIC measurement show that a high in-plane tensile strain at the substrate was observed around the front and side boundaries of the mussel plaque (Figure S10b and 11b). While the substrate deformation at the rear portion experienced compression in both in-plane principal directions, as shown in Figures S10b and c and Figures S11b and c. In addition, FE simulations suggest that interfaces at both substrates failed under NTGF, with debonding initiating from the rear portion and gradually spreading towards the front portion (Figure S10d and S11d). During the loading process, mussel plaques exhibit obvious deformation as the tensile load increases (Figure S10a and S11a). The geometrical sizes and positions of the compression and tension zones constantly change, with the compression zone expanding and shifting towards the front boundary (Figure S10b and 11b).

Figure S12 shows the deformation pattern of the “soft” substrate caused by the 90° tension. Similar to the “hard” substrate, mussel plaque experienced significant deformation at Point IV (Figure S12a). The distribution of the maximum in-plane strain  $\varepsilon_{max}$  around the rear portion exhibits a ring pattern with compression in the interior and tension in the exterior (Figure S12b), and the minimum in-plane strain  $\varepsilon_{min}$  exhibits a circle pattern with high in-plane compression in the centre (Figure S12c). Similar to the “hard” substrate, the in-plane principal strains were only detected at the rear portion of the plaque projection, while the substrate near the front portion of the plaque remained undeformed during the loading process (Figures S12b and c). The FE simulation indicated that debonding initiated at the thread projection position on the substrate under 90° tension, with the interface failing in NTGF mode (Figure S12d), similar to the failure mechanism observed under 45° tension.

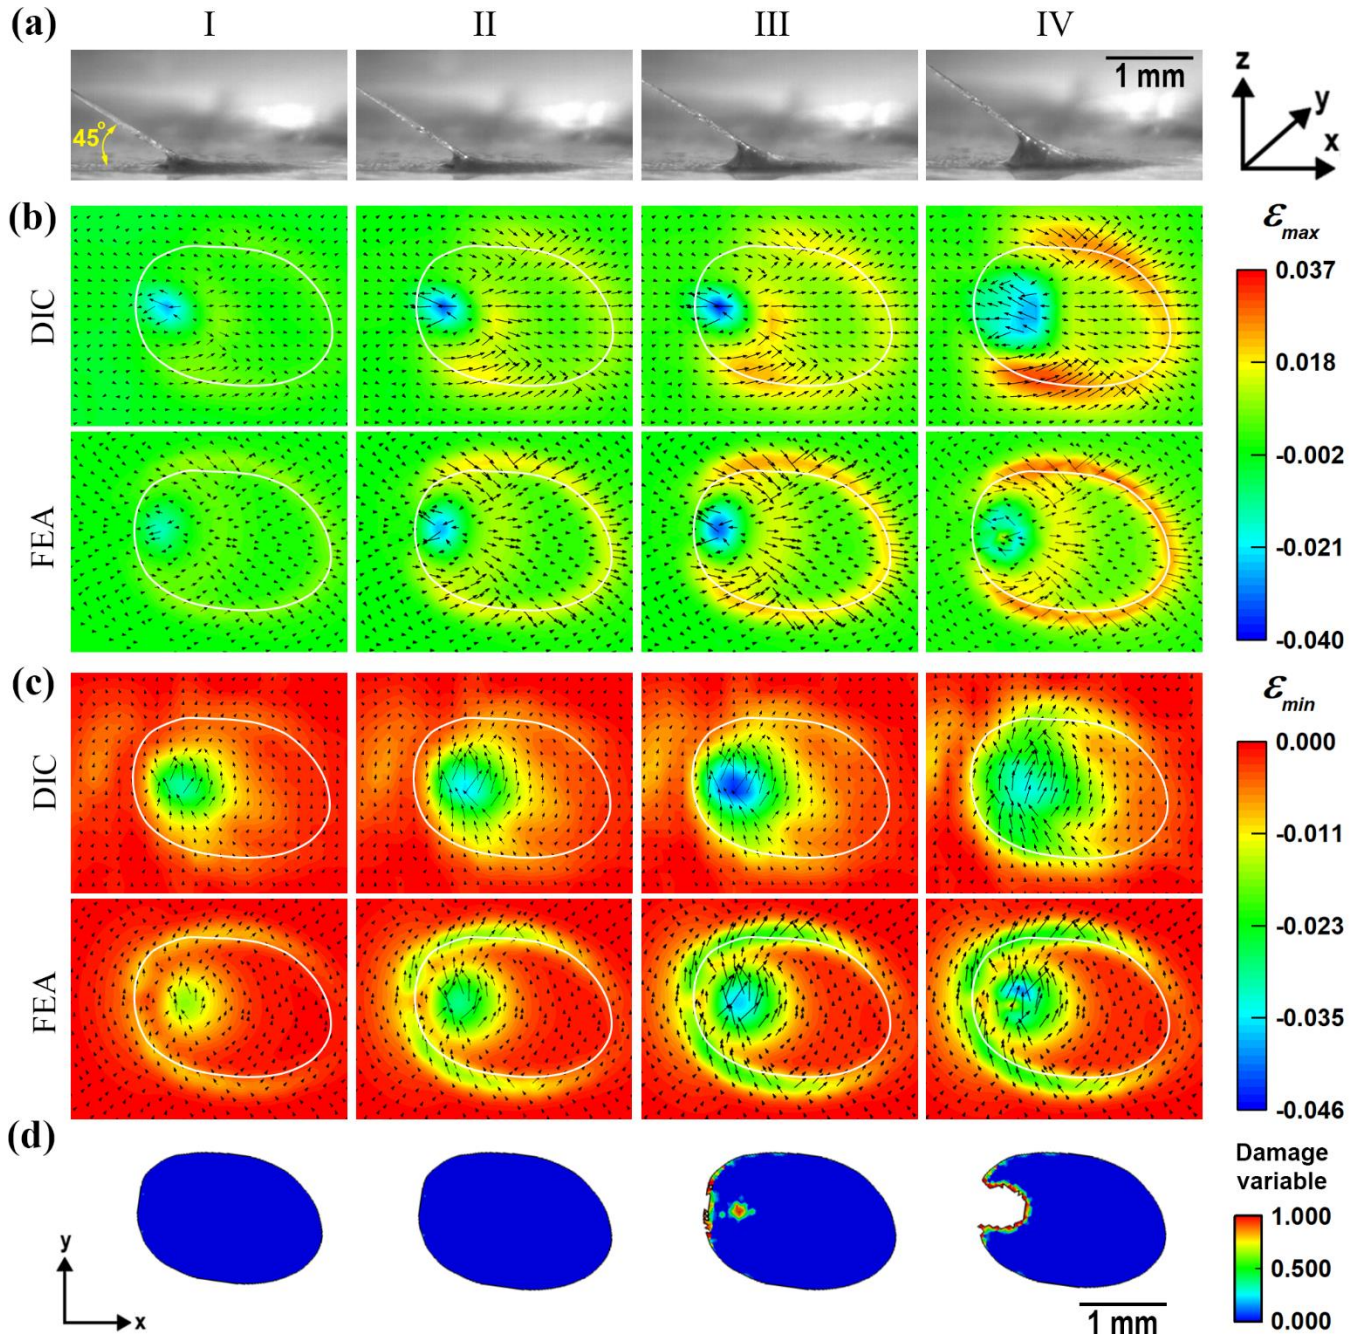

**Figure S10. Mussel plaque and substrate interaction on "hard" substrate under 45° tension.** (a) The side view of mussel plaque detaching under 45° tension. (b) and (c) Comparisons of DIC measurements and FE predictions showing the evolution of  $\epsilon_{max}$  and  $\epsilon_{min}$  on "hard" substrate, respectively. (d) the evolution of FE predicted cohesive failure on the "hard" substrate. Note that an obvious cohesive failure was observed at Point IV. The contour in white colour indicates the edge of the real mussel plaque.

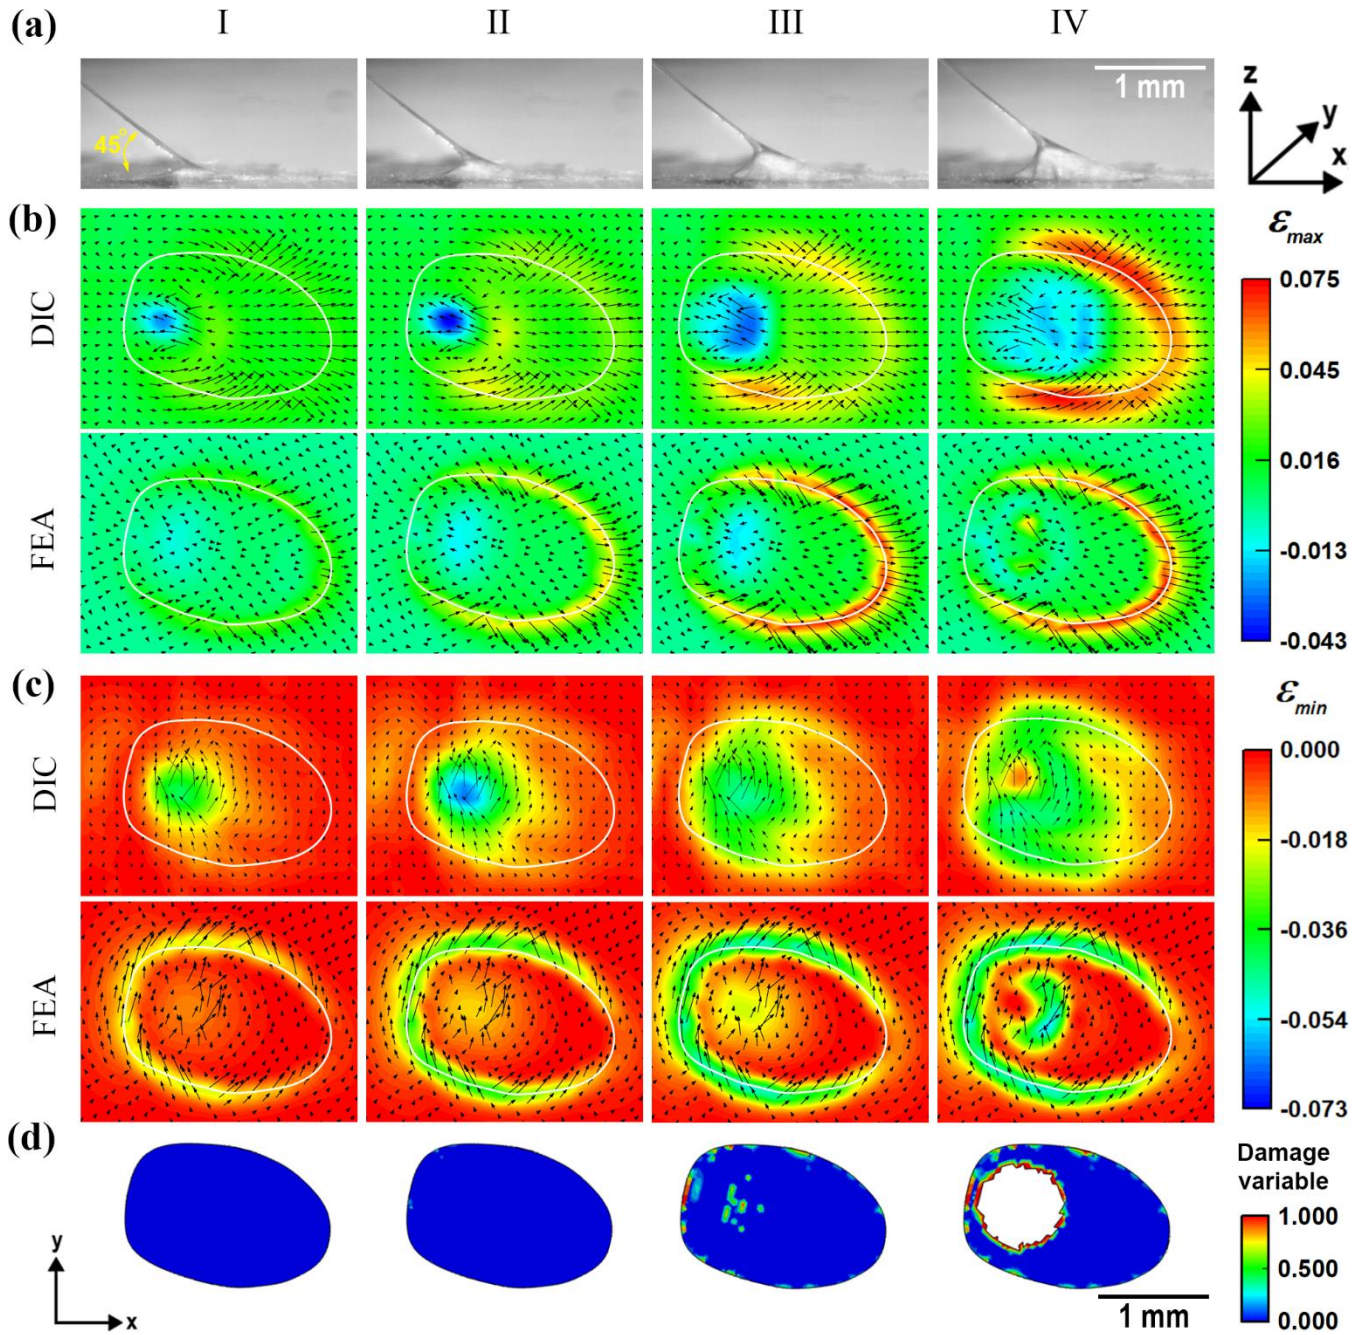

**Figure S11. Mussel plaque and substrate interaction on "soft" substrate under 45° tension.** (a) The side view of mussel plaque detaching under 45° tension. (b) and (c) Comparisons of DIC measurements and FE predictions showing the evolution of  $\epsilon_{max}$  and  $\epsilon_{min}$  on "hard" substrate, respectively. (d) the evolution of FE predicted cohesive failure on the "soft" substrate. Note that an obvious cohesive failure was observed at Point IV. The contour in white colour indicates the edge of the real mussel plaque.

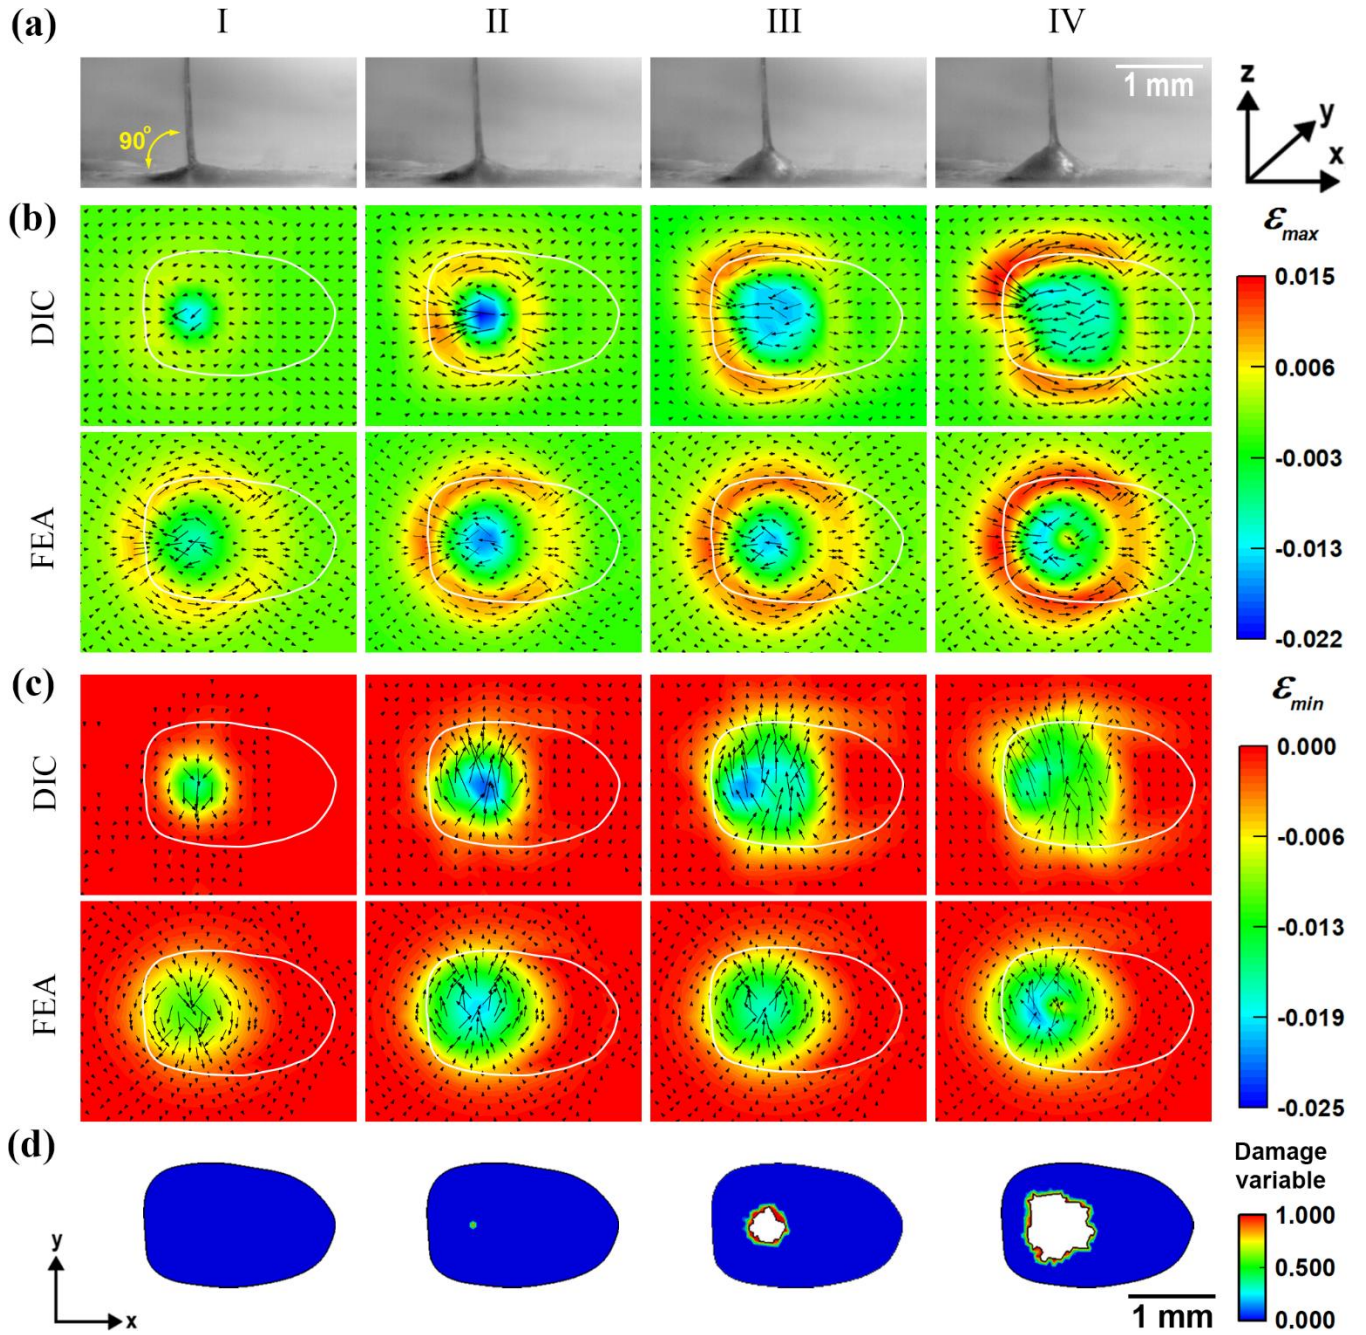

**Figure S12. Mussel plaque and substrate interaction on “soft” substrate under 90° tension.** (a) The side view of mussel plaque detaching under 90° tension. (b) and (c) Comparisons of DIC measurements and FE predictions showing the evolution of  $\epsilon_{max}$  and  $\epsilon_{min}$  on “soft” substrate, respectively. (d) the evolution of FE predicted cohesive failure on the “soft” substrate. Note that an obvious cohesive failure was observed at Point III. The contour in white colour indicates the edge of the real mussel plaque.

## References

1. ASTM D412-16. Standard test methods for vulcanized rubber and thermoplastic elastomers-tension. *ASTM Int. West Conshohocken, PA.* (2016).
2. Liu, M., Sun, J., Sun, Y., Bock, C. & Chen, Q. Thickness-dependent mechanical properties of polydimethylsiloxane membranes. *J. Micromech. Microeng* 19, 035028 (2009).
3. Y. Kwon, J. H. Bernstein, N. Cohen, and M. T. Valentine, On-Demand Manufacturing Capabilities of Mussels Enable Robust Adhesion to Geometrically Complex Surfaces, *ACS Biomater. Sci. Eng.* 7, 5099–5106 (2021).
4. S. Amini, S. Kolle, L. Petrone, O. Ahanotu, S. Sunny, C. N. Suto, S. Hoon, L. Cohen, J. C. Weaver, J. Aizenberg, et al., Preventing mussel adhesion using lubricant-infused materials, *Science* 357, 668–673 (2017).
5. T. Kang, X. Banquy, J. Heo, C. Lim, N. A. Lynd, P. Lundberg, D. X. Oh, H.-K. Lee, Y.-K. Hong, D. S. Hwang, et al., Mussel-inspired anchoring of polymer loops that provide superior surface lubrication and antifouling properties, *ACS Nano* 10, 930–937 (2016).
6. Schindelin, J., Arganda-Carreras, I., Frise, E., Kaynig, V., Longair, M., Pietzsch, T., ... & Cardona, A. (2012). Fiji: an open-source platform for biological-image analysis. *Nat. Methods*, 9(7), 676-682.
